# Supplementary material for: Explaining Anomalies in Groups with Characterizing Subspace Rules
Source: arXiv:1708.05929 source file (2018-05-02)
Supplement: Supplementary file 1 [file 070appendix.tex]

\setcounter{section}{0}

%\vspace{0.1in}

\section{\large{Extension to  Mixed-type features}}
\label{sec:extend}

Step I: use histograms

Step II: for converting a hyper-rectangle with mixed features,
first filter out all points that do not match any of categorical feature values,
 hyper-ellipsoid transformation on the  (normal and anomalous) points in the numerical subspace.

Step III: encoding scheme will change: for numerical subspace, submit 
 center and radius;  for each categorical feature, submit the value it takes in its domain.
